# Supplementary material for: How to write a coequation
Source: arXiv:2109.11967 source file (2021-09-24)
Supplement: Supplementary file 1 [file appendix.tex]

\section{Proofs}
